# Supplementary material for: New Boys and Girls in Phosphorene Family from Gene Recombination: Different from Parents, Excellent than Parents
Source: arXiv:1602.05734 source file (2016-02-18)
Supplement: Supplementary file 1 [file supplementary.pdf]

Supplementary for “New Boys and Girls in Phosphorene Family from Gene Recombination: Different from Parents, Excellent than Parents”

Chaoyu He, ChunXiao Zhang, Tao Ouyang, Jin Li and Jianxin Zhong

Hunan Key Laboratory for Micro-Nano Energy Materials and Devices, Xiangtan University, Hunan 411105, P. R. China;

School of Physics and Optoelectronics, Xiangtan University, Xiangtan 411105, China.

Here we provide a supplementary file including 1) perspective crystalline views of **η-P, θ-P, G1, G2, G3, B1** and **B2** from different directions, 2) testing results based on allotrope **G1** and black **α-P** for cutoff energy and K-mesh, 3) crystal structures, relative energies, surface work functions, band gaps and band structures of phosphorene allotropes in categories 4-7, 3-12, 4-8, 5-8 and 5-7, 4) phonon band structures and density of states for allotropes **G1, G2, G3, B1** and **B2**, 5) electronic band structures of allotropes **η-P, θ-P**, **G2, G3, B1** and **B2**, 6) as well as lattice constants and atomic positions for **G1, G2, G3, B1** and **B2** in format of VASP-POSCAR.

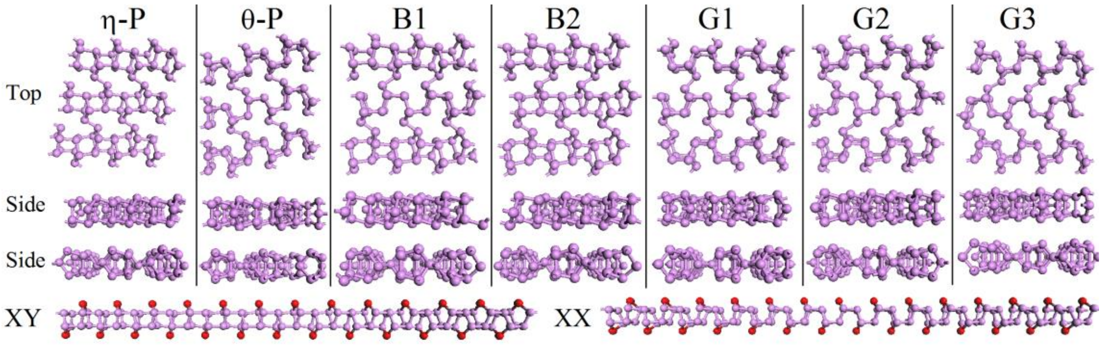


**Fig. S1.** Perspective top and side views of allotrope **η-P, θ-P, B1, B2, G1, G2** and **G3** and the corresponding **XY** and **XX** gene segments are shown.

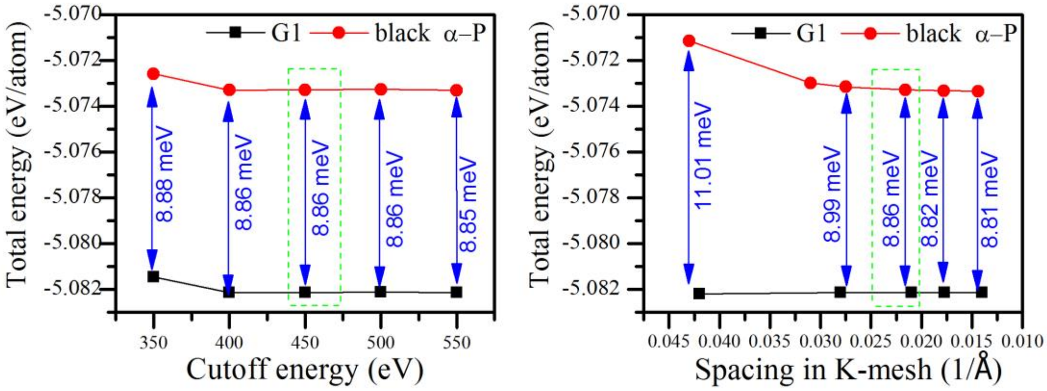


**Fig. S2.** Testing results based on allotrope **G1** and black **α-P**: dependence of total energy on cutoff energy (left) and on sample K-mesh (right).

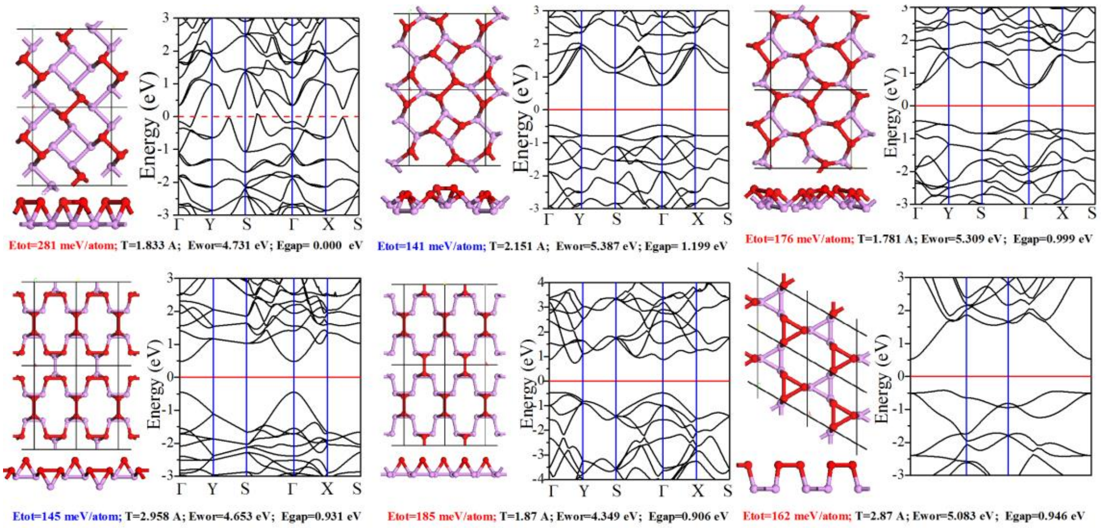


**Fig. S3** Crystal structures, relative energies (respect to **α-P**, meV/atom ), surface work functions, band gaps and band structures of phosphorene allotropes in categories 4-7 (top three) and 3-12 (down three).

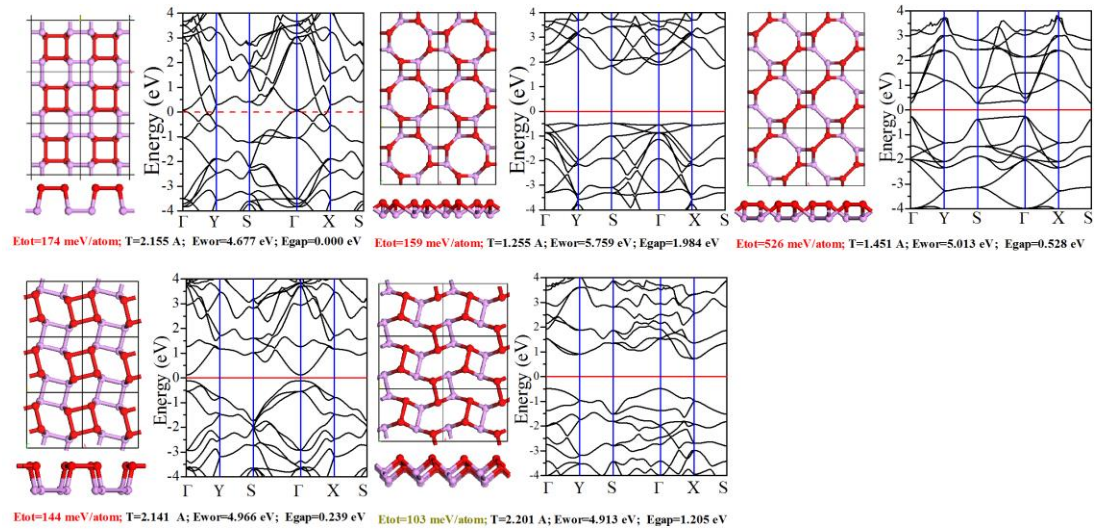


**Fig. S4** Crystal structures, relative energies (respect to **α-P**, meV/atom), surface work functions, band gaps and band structures of phosphorene allotropes in category 4-8.

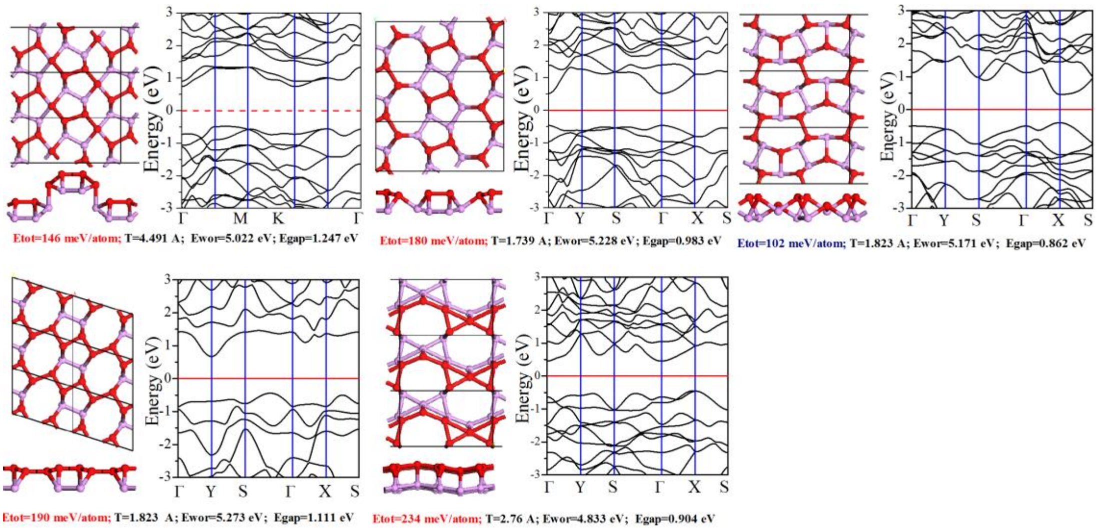


**Fig. S5** Crystal structures, relative energies (respect to **α-P**, meV/atom), surface work functions, band gaps and band structures of phosphorene allotropes in category 5-8.

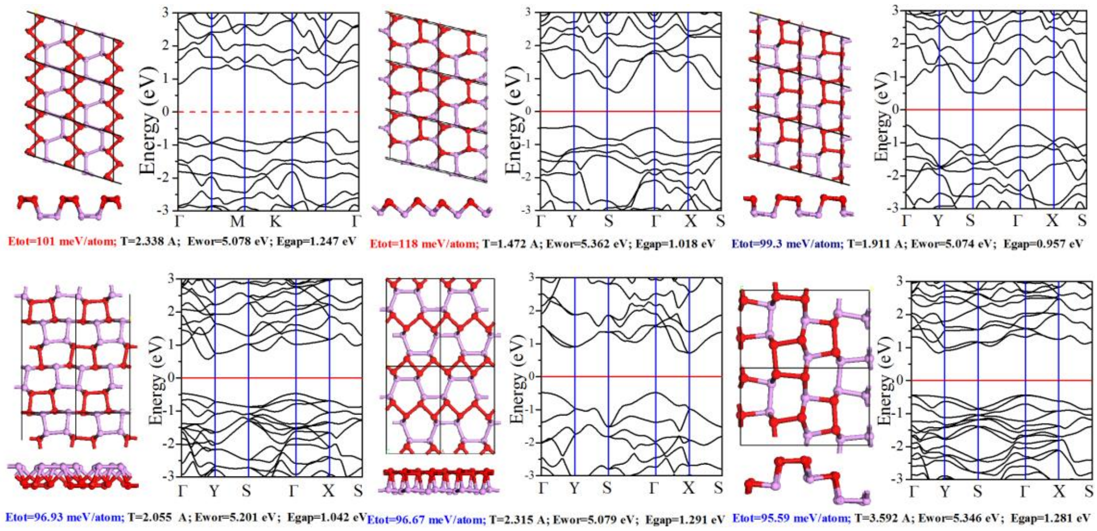


**Fig. S6** Crystal structures, relative energies (respect to **α-P**, meV/atom), surface work functions, band gaps and band structures of phosphorene allotropes in category 5-7.

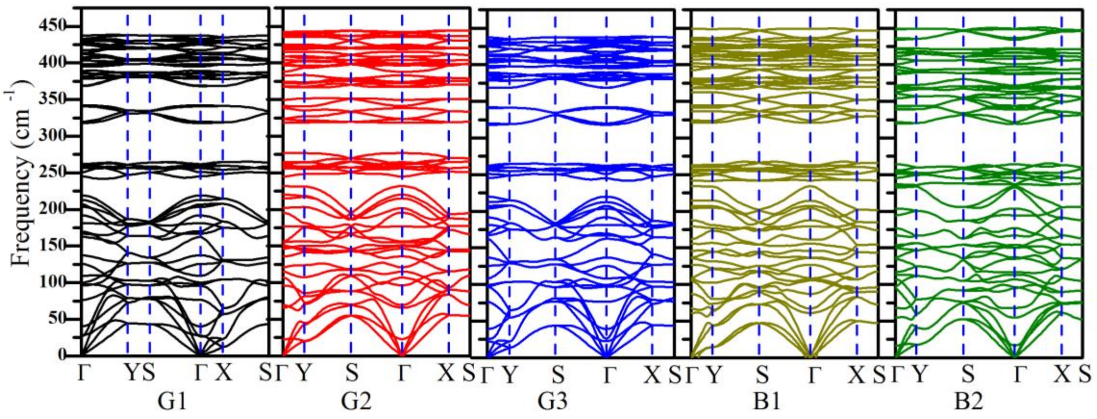


**Fig. S7.** Phonon band structures of allotropes **G1, G2, G3, B1** and **B2**.

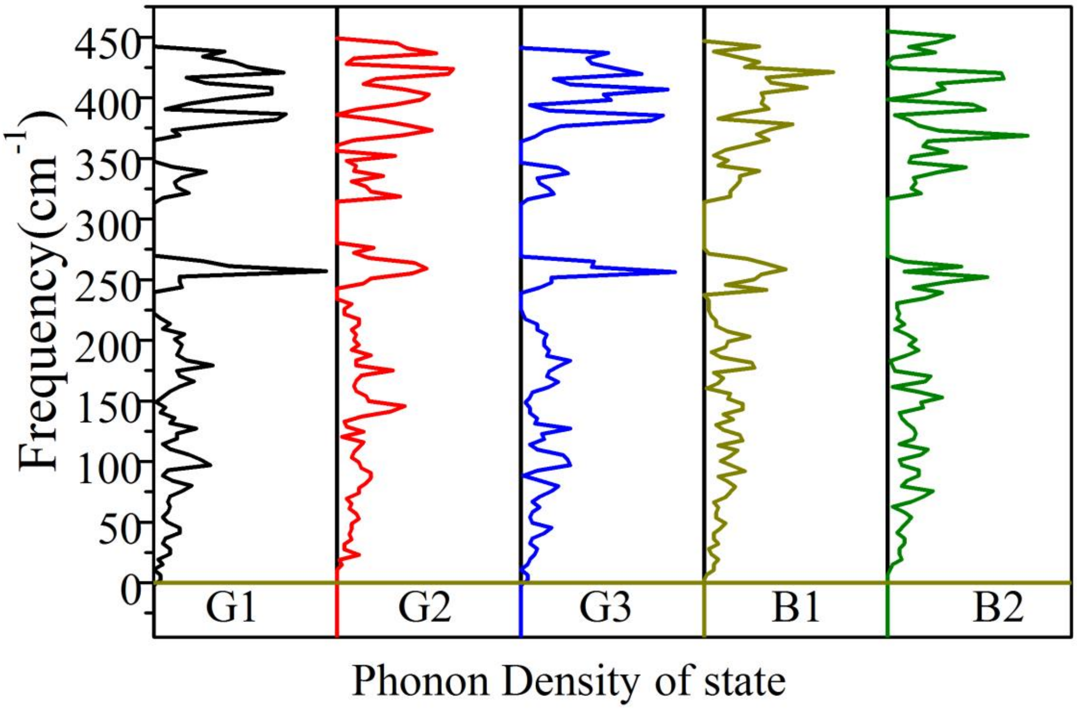


**Fig.S8.** Phonon density of states of allotropes **G1, G2, G3, B1** and **B2.**

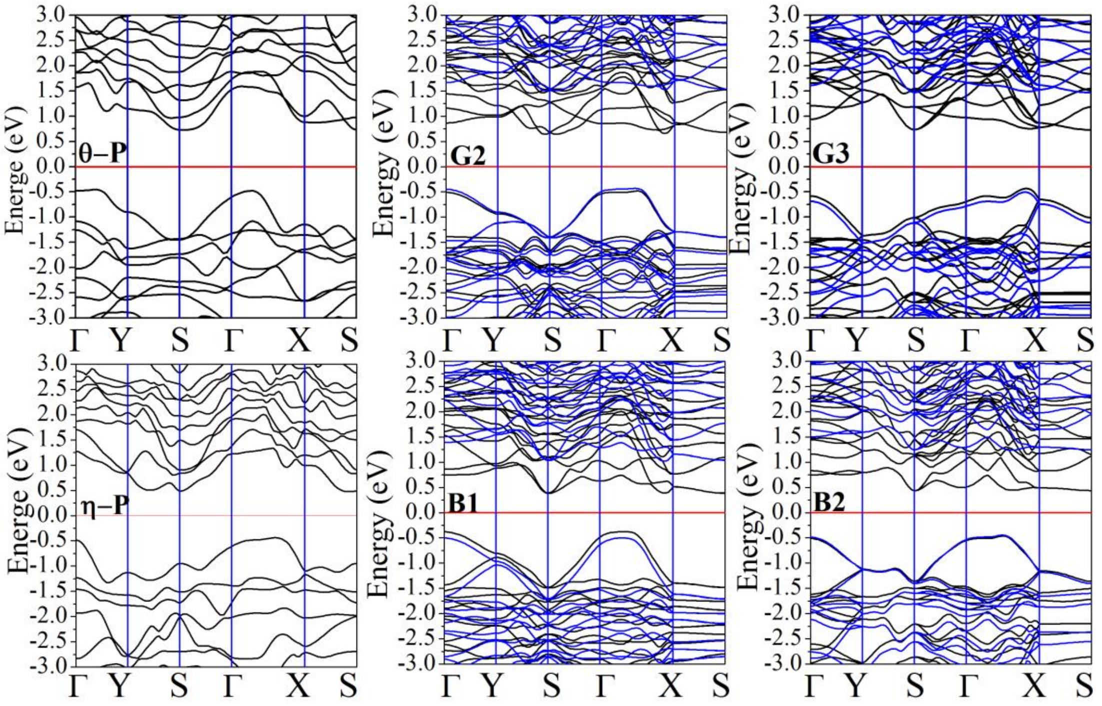


**Fig. S9.** Electronic band structures of allotropes **η-P**, **θ-P**, **G2, G3, B1** and **B2**, black solid lines are calculated form DFT method, blue solid lines are calculated form HSE06 method.

%******************************************************************************

**Optimized POSCARS：**

```
System G1
   1.00000000000000
     11.8497072543818174    0.0000000000000000    0.0000000000000000
      0.0000000000000000    5.7916016020632508    0.0000000000000000
      0.0000000000000000    0.0000000000000000   21.1810720377811670
   P
     20
Selective dynamics
Direct
  0.6674278580683116  0.9937482328743141  0.5821008870914718   T   T   T
  0.3325721419316884  0.0062517671256859  0.5821008870914718   T   T   T
  0.8325721419316884  0.4937482328743141  0.4178991129085283   T   T   T
  0.1674278580683116  0.5062517671256859  0.4178991129085283   T   T   T
  0.3325721419316884  0.0062517671256859  0.4178991129085283   T   T   T
  0.6674278580683116  0.9937482328743141  0.4178991129085283   T   T   T
  0.1674278580683116  0.5062517671256859  0.5821008870914718   T   T   T
  0.8325721419316884  0.4937482328743141  0.5821008870914718   T   T   T
  0.6631147558172339  0.6206314080143436  0.4461998348710229   T   T   T
  0.3368852441827661  0.3793685919856565  0.4461998348710229   T   T   T
  0.8368852441827661  0.1206314080143435  0.5538001651289770   T   T   T
  0.1631147558172339  0.8793685919856564  0.5538001651289770   T   T   T
  0.3368852441827661  0.3793685919856565  0.5538001651289770   T   T   T
  0.6631147558172339  0.6206314080143436  0.5538001651289770   T   T   T
  0.1631147558172339  0.8793685919856564  0.4461998348710229   T   T   T
  0.8368852441827661  0.1206314080143435  0.4461998348710229   T   T   T
  0.9289683807195661  0.6306473839456462  0.5000000000000000   T   T   T
  0.0710316192804339  0.3693526160543609  0.5000000000000000   T   T   T
  0.5710316192804339  0.1306473839456391  0.5000000000000000   T   T   T
  0.4289683807195661  0.8693526160543538  0.5000000000000000   T   T   T
```

```
System G2
   1.00000000000000
    18.5623619723813569    0.0000000000000000    0.0000000000000000
     0.0000000000000000   12.1435036394426898    0.0000000000000000
     0.0000000000000000    0.0000000000000000    5.5320161397083076
   P
    20
Selective dynamics
Direct
  0.4389034510607487  0.0768578317232911  0.2506805855257240   T   T   T
  0.5930558818960556  0.0918940186896764  0.8589122431537078   T   T   T
  0.4383371845256410  0.5772584874972573  0.9943084855694042   T   T   T
  0.5935121840608411  0.5925084930593418  0.6045240930848718   T   T   T
  0.5610965489392512  0.9231421682767090  0.7506805855257240   T   T   T
  0.4069441181039445  0.9081059813103236  0.3589122431537078   T   T   T
  0.5616628154743588  0.4227415125027428  0.4943084855694043   T   T   T
  0.4064878159391589  0.4074915069406578  0.1045240930848721   T   T   T
  0.4389034510607487  0.9231421682767090  0.7506805855257240   T   T   T
  0.5930558818960556  0.9081059813103236  0.3589122431537078   T   T   T
  0.4383371845256410  0.4227415125027428  0.4943084855694043   T   T   T
  0.5935121840608411  0.4074915069406578  0.1045240930848721   T   T   T
  0.5610965489392512  0.0768578317232911  0.2506805855257240   T   T   T
  0.4069441181039445  0.0918940186896764  0.8589122431537078   T   T   T
  0.5616628154743588  0.5772584874972573  0.9943084855694042   T   T   T
  0.4064878159391589  0.5925084930593418  0.6045240930848718   T   T   T
  0.5000000000000000  0.8041254435926182  0.2327540503400634   T   T   T
  0.5000000000000000  0.2947510383812398  0.0775795017743900   T   T   T
  0.5000000000000000  0.1958745564073820  0.7327540503400636   T   T   T
  0.5000000000000000  0.7052489616187604  0.5775795017743901   T   T   T
System G3
   1.00000000000000
    12.2803614276504671    0.0000000000000000    0.0000000000000000
     0.0000000000000000    5.5331090156098393    0.0000000000000000
     0.0000000000000000    0.0000000000000000   21.3931069495732125
   P
    20
Selective dynamics
Direct
  0.6551234699830537  0.8143128235714165  0.5806938014994544   T   T   T
  0.3448765300169465  0.1856871764285834  0.5806938014994544   T   T   T
  0.8448765300169463  0.3143128235714167  0.4193061985005458   T   T   T
  0.1551234699830536  0.6856871764285835  0.4193061985005458   T   T   T
  0.3448765300169465  0.1856871764285834  0.4193061985005458   T   T   T
  0.6551234699830537  0.8143128235714165  0.4193061985005458   T   T   T
  0.1551234699830536  0.6856871764285835  0.5806938014994544   T   T   T
  0.8448765300169463  0.3143128235714166  0.5806938014994544   T   T   T
  0.6775458851112961  0.4250302609288193  0.4465800698927901   T   T   T
  0.3224541148887037  0.5749697390711808  0.4465800698927901   T   T   T
  0.8224541148887039  0.9250302609288192  0.5534199301072099   T   T   T
  0.1775458851112963  0.0749697390711807  0.5534199301072099   T   T   T
  0.3224541148887037  0.5749697390711808  0.5534199301072099   T   T   T
  0.6775458851112961  0.4250302609288193  0.5534199301072099   T   T   T
  0.1775458851112963  0.0749697390711807  0.4465800698927901   T   T   T
  0.8224541148887039  0.9250302609288192  0.4465800698927901   T   T   T
  0.9603328107196692  0.3188941971824753  0.5000000000000000   T   T   T
  0.0396671892803310  0.6811058028175246  0.5000000000000000   T   T   T
  0.5396671892803308  0.8188941971824754  0.5000000000000000   T   T   T
  0.4603328107196690  0.1811058028175244  0.5000000000000000   T   T   T
```

```
System B1
   1.00000000000000
     19.1312388783536633    -0.0706784377989201     0.6346074277648454
     -0.0515090401905567    12.1745991397313453     0.0007561785948758
      0.2411912850221304    -0.0002427830349709     5.5335055750747122
   P
     20
Selective dynamics
Direct
  0.5493584107191866  0.6114643279904802  0.8403122477026034   T   T   T
  0.4019857320287569  0.6239520181615360  0.2796495750627784   T   T   T
  0.4302839604977734  0.4548209495929588  0.3779599736287172   T   T   T
  0.5830850032620838  0.4458481114647951  0.7170777445776184   T   T   T
  0.5494610045328241  0.4544851375332578  0.3402548137324877   T   T   T
  0.4020910157431630  0.4379792895451057  0.7795009723287470   T   T   T
  0.4301756086670223  0.6078643319871262  0.8780726308627630   T   T   T
  0.5830543809020036  0.6209906979371382  0.2170680825561708   T   T   T
  0.4947456405758649  0.7257644393743867  0.3714059416396344   T   T   T
  0.4948991052698061  0.3385938628461270  0.8711890382786686   T   T   T
  0.4340728658780099  0.1126493505669539  0.1021252057600446   T   T   T
  0.5773559054701659  0.1282547189134263  0.4643247780416134   T   T   T
  0.5515843121977336  0.1092158709651543  0.0673667270186677   T   T   T
  0.4005610865107658  0.1157137240261712  0.7203745518187521   T   T   T
  0.4809047319527467  0.8328521856748897  0.0434688791227489   T   T   T
  0.4339801005262949  0.9500670788994651  0.6021482120624366   T   T   T
  0.5771965692265423  0.9375279314059394  0.9643707057712290   T   T   T
  0.5514912293949504  0.9559831519708835  0.5673607501032732   T   T   T
  0.4004219532801298  0.9463363996057937  0.2204704328176073   T   T   T
  0.4811500270120166  0.2309564682672054  0.5431964490358290   T   T   T
System B2
   1.00000000000000
     19.8574272632984403     0.0000000000000000     0.0442035043417624
      0.0000000000000000    12.2873136582989222     0.0000000000000000
      0.1641709753438675     0.0000000000000000     5.4397149262477393
   P
     20
Selective dynamics
Direct
  0.4407281317667481  0.8217300949818158  0.1355137565165119   T   T   T
  0.5880264298729068  0.8349694711713116  0.5049629371439202   T   T   T
  0.5535308659630670  0.8286424558764526  0.1176544013900302   T   T   T
  0.4186250596803767  0.8505998454028328  0.7261646287533096   T   T   T
  0.5124791110625977  0.5474452422656969  0.1713965121798033   T   T   T
  0.5592718682332520  0.3217300949818159  0.3644862434834880   T   T   T
  0.4119735701270932  0.3349694711713120 -0.0049629371439200   T   T   T
  0.4464691340369331  0.3286424558764529  0.3823455986099698   T   T   T
  0.5813749403196234  0.3505998454028327  0.7738353712466904   T   T   T
  0.4875208889374025  0.0474452422656970  0.3286034878201967   T   T   T
  0.5592718682332520  0.1782699050181842  0.8644862434834882   T   T   T
  0.4119735701270932  0.1650305288286882  0.4950370628560800   T   T   T
  0.4464691340369331  0.1713575441235472  0.8823455986099699   T   T   T
  0.5813749403196234  0.1494001545971672  0.2738353712466905   T   T   T
  0.4875208889374025  0.4525547577343030  0.8286034878201967   T   T   T
  0.4407281317667481  0.6782699050181842  0.6355137565165118   T   T   T
  0.5880264298729068  0.6650305288286884  0.0049629371439200   T   T   T
  0.5535308659630670  0.6713575441235474  0.6176544013900301   T   T   T
  0.4186250596803767  0.6494001545971672  0.2261646287533025   T   T   T
  0.5124791110625977  0.9525547577343031  0.6713965121798033   T   T   T
```
